# Supplementary material for: A Study of the Mathematics of Deep Learning
Source: arXiv:2104.14033 source file (2021-04-28)
Supplement: Supplementary file 2 [file Appendix_Neural_Training.tex]

\chapter*{\vspace{10pt} Appendix To Chapter \ref{chaptrain}}\label{app:train} %

\section{Reviewing a variant of the Azuma-Hoeffding Inequality}

\begin{theorem}\label{AHSM} 
Suppose we have a real valued discrete stochastic process given as, $\{X_0,X_i,\ldots\}$ and the following properties hold,

\begin{itemize}
    \item $X_0$ is a constant  
    \item (The bounded difference property) $\forall i =0,1,\ldots$ $\exists c_i >0$ s.t $\vert X_i - X_i \vert \leq c_i$
    \item (The super-martingale property) $\forall i =0,1,\ldots$, $\E \Big [ X_i - X_{i-1} \mid {\cal F}_{i-1} \Big ] \leq 0$ with ${\cal F}_{i-1} = \sigma \Big ( \Big \{ X_0,\ldots,X_{i-1} \Big \} \Big )$
\end{itemize}

Then for any $\lambda >0$ and a positive integer $n$ we have the following concentration inequality, 

\[ \mathbb{P} \Big [ X_n - X_0 \geq \lambda  \Big ] \leq e^{-\frac{1}{2} \frac{\lambda^2}{\sum_{i=1}^n c_i^2} } \]
\end{theorem}

\begin{proof}
We note that for any $c,t >0$, the function $f(x) = e^{tx}$ lies below the straight line connecting the two points $(-c,f(-c))$ and $(c,f(c))$. This gives the inequality, $e^{tx} \leq e^{-tc} + \Big ( \frac{e^{tc} - e^{-tc}}{2c} \Big ) (x + c)$. This simplifies to, 

\begin{align}\label{basic}
e^{tx} \leq \frac{1}{2c} (e^{tc} - e^{-tc})x + \Big ( \frac{e^{tc} + e^{-tc}}{2} \Big )    
\end{align}

Note that the above inequality holds only when $\vert x \vert \leq c$

Now we can invoke the bounded difference property of $\vert X_i - X_i \vert \leq c_i$ and use equation \ref{basic} with $x = X_i - X_i$ and $c = c_i$ to get,  

\[ \E \Big [ e^{t(X_i - X_{i-1})} \mid {\cal F}_{i-1}  \Big ] \leq \E \Big [ \frac{e^{tc_i} - e^{-tc_i}}{2c_i} \Big (X_i - X_{i-1}\Big )  + \Big ( \frac{e^{tc_i} + e^{-tc_i}}{2} \Big )     \mid {\cal F}_{i-1} \Big ] \leq \frac{e^{tc_i} + e^{-tc_i}}{2} \] 

The last inequality follows from the given property that, $\E \Big [ X_i - X_{i-1} \mid {\cal F}_{i-1} \Big ] \leq 0$

Now we invoke the inequality $\frac{e^x + e^{-x}}{2} \leq e^{\frac {x^2}{2}}$ on the RHS above to get, 

\[ \E \Big [ e^{t(X_i - X_{i-1})} \mid {\cal F}_{i-1}  \Big ] \leq e^{\frac {t^2 c_i^2}{2} } \]

Further since $X_{i-1}$ is ${\cal F}_{i-1}$ measurable we can write the above as, 
$\E \Big [ e^{tX_i}  \mid {\cal F}_{i-1}  \Big ] \leq e^{tX_{i-1}} e^{\frac {t^2 c_i^2}{2} }$

Now we recurse the above as follows, 

\[ \E \Big [ e^{tX_n} \Big ] = \E \Big [ \E \Big [ e^{tX_n} \mid {\cal F}_{n-1} \Big ] \Big ] \leq \E \Big [  e^{\frac{t^2 c_n^2}{2}} e^{tX_{n-1}} \Big ] = e^{\frac{t^2 c_n^2}{2}} \E \Big [ e^{tX_{n-1}} \Big ] \ldots \leq \prod_{i=1}^n e^{\frac {t^2 c_i^2}{2}} \E [ e^{tX_0} ]  \]

Now invoking that $X_0$ is a constant we can rewrite the above as, $\E \Big [ e^{t(X_n-X_0)} \Big ] \leq e^{\frac{t^2}{2} \sum_{i=1}^n c_i^2}$

Hence for any $\lambda >0$ we have by invoking the above,

\[ \mathbb{P} \Big [ X_n - X_0 \geq \lambda  \Big ] = \mathbb{P} \Big [ e^{t(X_n - X_0)} \geq e^{t\lambda} \Big ] \leq e^{-t\lambda} \E \Big [ e^{t(X_n - X_0)} \Big ] \leq e^{-t\lambda}e^{\frac{t^2}{2} \sum_{i=1}^n c_i^2}  \]

Now choose $t = \frac{\lambda}{\sum_{i=1}^n c_i^2}$ and we get, 
$\mathbb{P} \Big [ X_n - X_0 \geq \lambda  \Big ] \leq e^{-\frac{1}{2} \frac{\lambda^2}{\sum_{i=1}^n c_i^2} }$

\end{proof}

\section{Proof of Lemma \ref{stepdecrease}}\label{app:glmtronstep}
\begin{proof}
We observe that, 
\begin{align}\label{main} 
\nonumber \norm{\w_t - \w}^2 - \norm{\w_{t+1} - \w}^2    &= \norm{\w_t - \w}^2 - \norm{\Big ( \w_{t} + \frac {1}{S} \sum_{i=1}^S \Big (y_i - \sigma (\langle \w_t , \x_i\rangle) \Big )\x_i \Big ) - \w}^2\\
\nonumber &= -\frac{2}{S} \sum_{i=1}^S \Big \langle \Big (y_i - \sigma (\langle \w_t , \x_i\rangle) \Big)\x_i, \w_t - \w \Big  \rangle - \norm{\frac{1}{S}\sum_{i=1}^S \Big ( y_i - \sigma (\langle \w_t , \x_i\rangle ) \Big )\x_i}^2\\
&= \frac{2}{S} \sum_{i=1}^S \Big ( y_i - \sigma (\langle \w_t , \x_i\rangle) \Big ) \Big (\langle \w,\x_i \rangle  - \langle \w_t , \x_i \rangle \Big ) - \norm{\frac{1}{S}\sum_{i=1}^S \Big (y_i - \sigma (\langle \w_t , \x_i\rangle) \Big ) \x_i}^2
\end{align}

Analyzing the first term in the RHS above we get, 

\begin{align*} 
&\frac{2}{S} \sum_{i=1}^S \Big ( y_i - \sigma (\langle \w_t , \x_i\rangle) \Big ) \Big (\langle \w,\x_i \rangle  - \langle \w_t , \x_i \rangle \Big ) = \frac{2}{S} \sum_{i=1}^S \Big (y_i - \sigma (\langle \w, \x_i \rangle ) + \sigma  (\langle \w, \x_i \rangle) - \sigma (\langle \w_t , \x_i\rangle) \Big ) \Big (\langle \w,\x_i \rangle  - \langle \w_t , \x_i \rangle \Big )\\
&= \frac{2}{S} \sum_{i=1}^S \Big \langle \Big (y_i - \sigma (\langle \w, \x_i \rangle ) \Big )\x_i, \w - \w_t \Big \rangle 
+   \frac{2}{S} \sum_{i=1}^S \Big (\sigma (\langle \w, \x_i \rangle) - \sigma (\langle \w_t , \x_i\rangle) \Big ) \Big ( \langle \x_i, \w \rangle - \langle \x_i , \w_t \rangle \Big )\\
&\geq - 2\eta W + \frac{2}{S} \sum_{i=1}^S  \Big ( \sigma (\langle \w, \x_i \rangle)  - \sigma (\langle \w_t , \x_i\rangle) \Big ) \Big ( \langle \x_i, \w \rangle - \langle \x_i , \w_t \rangle \Big)
\end{align*} 

In the first term above we have invoked the definition of $\eta$ and $W$ given in the Lemma. Further since we are given that $\sigma$ is non-decreasing and $L-$Lipschitz, we have for the second term in the RHS above, 

$\frac{2}{S} \sum_{i=1}^S  \Big ( \sigma (\langle \w, \x_i \rangle)  - \sigma (\langle \w_t , \x_i\rangle) \Big ) \Big ( \langle \x_i, \w \rangle - \langle \x_i , \w_t \rangle \Big)  \geq \frac{2}{SL} \sum_{i=1}^S  \Big ( \sigma (\langle \w, \x_i \rangle) - \sigma (\langle \w_t , \x_i\rangle) \Big )^2 =: \frac{2}{L} \tilde{L}_S (h_t)$

Thus together we have, 

\begin{eqnarray}\label{main1}
%\rightindent \text{Thus together we have,}\\ 
\frac{2}{S} \sum_{i=1}^S \Big (y_i - \sigma (\langle \w_t , \x_i\rangle) \Big ) \Big (\langle \w,\x_i \rangle  - \langle \w_t , \x_i \rangle \Big ) \geq -2\eta W  + \frac{2}{L} \tilde{L}_S (h_t) 
\end{eqnarray}

Now we look at the second term in the RHS of equation \ref{main} and that gives us, 

\begin{align}\label{main2}
\nonumber &\norm{\frac{1}{S}\sum_{i=1}^S \Big (y_i - \sigma (\langle \w_t , \x_i\rangle) \Big )\x_i}^2 = \norm{\frac{1}{S}\sum_{i=1}^S \Big (y_i - \sigma (\langle \w , \x_i\rangle) + \sigma(\langle \w , \x_i\rangle) - \sigma(\langle \w_t , \x_i\rangle ) \Big )\x_i}^2\\
\nonumber &\leq \norm{\frac{1}{S}\sum_{i=1}^S \Big (y_i - \sigma (\langle \w , \x_i\rangle) \Big )\x_i}^2 + 2 \norm{\frac{1}{S}\sum_{i=1}^S \Big (y_i - \sigma(\langle \w , \x_i\rangle) \Big)\x_i} \times \norm{\frac{1}{S}\sum_{i=1}^S \Big (\sigma(\langle \w , \x_i\rangle) - \sigma(\langle \w_t , \x_i\rangle) \Big)\x_i}\\
\nonumber &+ \norm{\frac{1}{S}\sum_{i=1}^S \Big (\sigma(\langle \w , \x_i\rangle) - \sigma(\langle \w_t , \x_i\rangle) \Big )\x_i}^2\\
 &\leq \eta^2 + 2\eta  \norm{\frac{1}{S}\sum_{i=1}^S \Big (\sigma(\langle \w , \x_i\rangle) - \sigma(\langle \w_t , \x_i\rangle) \Big)\x_i} + \norm{\frac{1}{S}\sum_{i=1}^S \Big (\sigma(\langle \w , \x_i\rangle) - \sigma(\langle \w_t , \x_i\rangle) \Big )\x_i}^2
\end{align}

Now by Jensen's inequality we have, 

$\norm{\frac{1}{S}\sum_{i=1}^S \Big (\sigma(\langle \w , \x_i\rangle) - \sigma(\langle \w_t , \x_i\rangle) \Big)\x_i}^2 \leq \frac{1}{S}\sum_{i=1}^S \Big (\sigma(\langle \w , \x_i\rangle) - \sigma(\langle \w_t , \x_i\rangle) \Big )^2 = \tilde{L}_S(h_t)$

And we have from the definition of $L$ and $W$,

\[ \norm{\frac{1}{S}\sum_{i=1}^S \Big ( \sigma(\langle \w , \x_i\rangle) - \sigma(\langle \w_t , \x_i\rangle) \Big )\x_i} \leq \frac{L}{S}\sum_{i=1}^S \norm{ \w - \w_t} \leq L \times W  \]

Substituting the above two into the RHS of equation \ref{main2} we have,

\begin{align}\label{main3} 
\norm{\frac{1}{S}\sum_{i=1}^S \Big (y_i - \sigma (\langle \w_t , \x_i\rangle) \Big )\x_i}^2 \leq \eta^2 + 2\eta LW + \tilde{L}_S(h_t)
\end{align} 

Now we substitute equations \ref{main1} and \ref{main3} into equation \ref{main} to get, 

\[  \norm{\w_t - \w}^2 - \norm{\w_{t+1} - \w}^2  \geq \Big ( -2\eta W  + \frac{2}{L} \tilde{L}_S (h_t) \Big ) -(\eta^2 + 2\eta LW + \tilde{L}_S(h_t))    \] 

The above simplifies to the inequality we claimed in the lemma i.e,

\[ \norm{\w_{t+1} - \w}^2  \leq  \norm{\w_t - \w}^2 - \Big ( \frac 2 L -1  \Big )\tilde{L}_S (h_t) + \Big ( \eta^2 + 2\eta W (L +1 )  \Big )  \] 

\end{proof} 

\section{Proof of Lemma \ref{NeuroTronD2FBSinglestepdecrease}}\label{app : NeuroTronD2FBSinglestepdecrease} 

\begin{proof}
We observe that, 
\begin{align}\label{mainN} 
\nonumber &\norm{\w_t - \w}^2 - \norm{\w_{t+1} - \w}^2 \\
\nonumber &= \norm{\w_t - \w}^2 - \norm{\Big ( \w_{t} + \frac {2\eta}{wS} \sum_{i=1}^S (y_i - f_{\w_t}(\x_i)) \M \x_i \Big ) - \w}^2\\
\nonumber &= -\frac{4 \eta}{wS} \sum_{i=1}^S \Big \langle \Big (y_i - f_{\w_t}( \x_i) \Big ) M \x_i, \w_t - \w \Big \rangle - \norm{\frac{2\eta}{wS}\sum_{i=1}^S \Big (y_i - f_{\w_t}( \x_i) \Big ) M\x_i}^2\\
&= \underbrace{-\frac{4 \eta }{wS} \sum_{i=1}^S \Big ( y_i - f_{\w_t}(\x_i) \Big ) \Big (\langle \w_t, M\x_i \rangle  - \langle \w , M\x_i \rangle \Big )}_{\text{\bf Term 1}} - \left ( \frac{2\eta}{w} \right )^2 \underbrace{\norm{\frac{1}{S}\sum_{i=1}^S \Big (y_i - f_{\w_t}(\x_i) \Big ) M \x_i}^2}_{\text{\bf Term 2}}
\end{align}

Now we shall try to lowerbound the RHS above. We achieve that in two steps that of finding a lowerbound on Term 1 and finding an upperbound on Term 2 as demarcated above

{\bf Lowerbound on ``Term 1" in the RHS of equation \ref{mainN}}

\begin{align}\label{cross}  
\nonumber &\text{Term 1 =} \frac{4 \eta }{wS} \sum_{i=1}^S \Big ( y_i - f_{\w_t}(\x_i) \Big ) \Big (\langle \w, \M\x_i \rangle  - \langle \w_t , \M\x_i \rangle \Big )\\
\nonumber &= \frac{4 \eta }{wS} \sum_{i=1}^S \Big (y_i - f_{\w}(\x_i) + f_{\w}(\x_i) - f_{\w_t}(\x_i)  \Big ) \Big (\langle \w, \M\x_i \rangle  - \langle \w_t , \M \x_i \rangle \Big )\\
\nonumber &= \frac{4 \eta }{wS} \sum_{i=1}^S \Big (y_i - f_{\w}(\x_i) \Big ) \Big \langle  \M \x_i, \w - \w_t \Big \rangle  \\
\nonumber &+  \frac{4 \eta }{wS} \sum_{i=1}^S  \Big ( f_{\w}(\x_i) - f_{\w_t}(\x_i) \Big )\Big  \langle \M\x_i, \w  -  \w_t \Big \rangle \\
&\geq - 4\frac{\eta \beta \norm{\w-\w_t}}{w}  + \frac{4 \eta }{wS} \sum_{i=1}^S  \Big ( f_{\w}(\x_i) - f_{\w_t}(\x_i)  \Big ) \Big  \langle \M\x_i, \w - \w_t \Big \rangle 
\end{align} 

To get the first term in the RHS above we have written $\frac{1}{S}\sum_{i=1}^S \Big (y_i - f_{\w}(\x_i) \Big ) \Big \langle  \M \x_i, \w - \w_t \Big \rangle = \frac{1}{S}\sum_{i=1}^S \Big (y_i - f_{\w}(\x_i) \Big ) ( \M \x_i)^\top \Big ( \w - \w_t \Big ) $ as $\p_1^\top \p_2$ for $\p_1, \p_2 \in \R^r$ given as, $\p_1 = \frac{1}{S}\sum_{i=1}^S \Big (y_i - f_{\w}(\x_i) \Big ) ( \M \x_i)$ and $\p_2 = \w - \w_t$. We invoke the definition of $\beta$ and $W$ as given in the Lemma and do reverse Cauchy-Schwarz inequality as, $\p_1^\top \p_2 \geq - \norm{\p_1}\norm{\p_2} \geq - \beta \norm{\w-\w_t}$. 

Now we invoke Lemma \ref{discretesym} to analyze the second term in the RHS of equation \ref{cross} and we get, 

\begin{align}
\nonumber &\frac{4 \eta }{wS} \sum_{i=1}^S \Big ( f_{\w}(\x_i) - f_{\w_t}(\x_i)  \Big ) \Big \langle \M\x_i, \w - \w_t \Big \rangle \\
\nonumber&=  \frac{4 \eta }{wS}  \sum_{i=1}^S \sum_{j=1}^w \Big \{  \sigma \Big ( \langle \A_j^\top \w , \x_i \rangle \Big ) -  \sigma \Big ( \langle \A_j^\top \w_t , \x_i \rangle \Big )  \Big \} \Big \langle \M\x_i, \w - \w_t \Big \rangle\\
\nonumber&= \frac{4 \eta }{wS} \sum_{j=1}^w \Big [  \sum_{i=1}^S \sigma \Big ( \langle \A_j^\top \w , \x_i \rangle \Big ) \Big \langle \M\x_i, \w - \w_t \Big \rangle    - \sum_{i=1}^S \sigma \Big ( \langle \A_j^\top \w_t , \x_i \rangle \Big ) \Big \langle \M\x_i, \w - \w_t \Big \rangle    \Big ]\\
\nonumber&= \frac{4 \eta (1+\alpha)}{2wS} \sum_{j=1}^w \Big [ \w^\top \Big ( \A_j \tilde{\Sigma}  \M^\top \Big )  (\w - \w_t) - \w_t^\top \Big ( \A_j \tilde{\Sigma}  \M^\top \Big )  (\w - \w_t)  \Big ]\\
&= \frac{4 \eta (1+\alpha)}{2S}  \Big [ (\w - \w_t)^\top \Big ( \bar{\A} \tilde{\Sigma}  \M^\top \Big )  (\w - \w_t) \Big ]
\end{align}

Substituting the above into the RHS of equation \ref{cross} we get,

\begin{align}\label{term1} 
    \nonumber \text{ Term 1} &= \frac{4 \eta }{wS} \sum_{i=1}^S \Big ( y_i - f_{\w_t}(\x_i) \Big ) \Big (\langle \w, \M\x_i \rangle  - \langle \w_t , \M\x_i \rangle \Big )\\
    &\geq  -4\frac{\eta \beta \norm{\w-\w_t}}{w}  + 4\frac{ \eta (1+\alpha)}{2S}  \Big [ (\w - \w_t)^\top \Big ( \bar{\A} \tilde{\Sigma}  \M^\top \Big )  (\w - \w_t) \Big ]
\end{align}

{\bf Upperbound on ``Term 2" in the RHS of equation \ref{mainN}}

\begin{align}\label{mainN2}
\nonumber \text{Term 2 } &= \norm{\frac{1}{S}\sum_{i=1}^S \Big (y_i - f_{\w_t}(\x_i) \Big ) \M \x_i}^2 = \norm{\frac{1}{S}\sum_{i=1}^S \Big (y_i - f_{\w}(\x_i) + f_{\w}(\x_i) - f_{\w_t}(\x_i) \Big )\M\x_i}^2\\
\nonumber &\leq \norm{\frac{1}{S}\sum_{i=1}^S \Big (y_i - f_{\w}(\x_i)) \Big ) \M\x_i}^2 + 2 \norm{\frac{1}{S}\sum_{i=1}^S \Big (y_i - f_{\w}(\x_i) \Big) \M\x_i} \times \norm{\frac{1}{S}\sum_{i=1}^S \Big ( f_{\w}(\x_i) - f_{\w_t}(\x_i) \Big) \M \x_i}\\
\nonumber &+ \norm{\frac{1}{S}\sum_{i=1}^S \Big (f_{\w}(\x_i) - f_{\w_t}(\x_i) \Big )\M\x_i}^2\\
 &\leq \beta ^2 + 2\beta  \norm{\frac{1}{S}\sum_{i=1}^S \Big ( f_{\w}(\x_i) - f_{\w_t}(\x_i) \Big)\M\x_i} + \norm{\frac{1}{S}\sum_{i=1}^S \Big (f_{\w}(\x_i) - f_{\w_t}(\x_i) \Big )\M\x_i}^2
\end{align}

Now by Jensen's inequality we have for the third term of the RHS above, 

\[ \norm{\frac{1}{S}\sum_{i=1}^S \Big ( f_{\w}(\x_i) - f_{\w_t}(\x_i) \Big ) \M \x_i}^2 \leq \frac{1}{S}\sum_{i=1}^S \Big (f_{\w}(\x_i) - f_{\w_t} (\x_i) \Big )^2 \norm{\M \x_i}^2 =  \frac{{\rm B}^2 \lambda_{\max} \Big ( \M^\top \M \Big ) }{S} \sum_{i=1}^S \Big (f_{\w}(\x_i) - f_{\w_t} (\x_i) \Big )^2 \]

In the above we have used for every $i$ the following relationships invoking the definition of the parameter {\rm B}, 
\[ \norm{\M \x_i}^2 = \x_i^\top (\M^\top \M) \x_i \leq \lambda_{\max} \Big ( \M^\top \M \Big ) \norm{\x_i}^2 \leq {\rm B}^2 \lambda_{\max} \Big ( \M^\top \M \Big )  \]

% For any positive semi-definite matrix $\A$, the quadratic form $\x^T\A\x$ has bounds based on the eigenvalue as, 
%     \[
%     \lambda_{\min}(\A) \cdot \norm{x}^2 \leq \x^T \A x \leq \lambda_{\max}(\A) \cdot \norm{x}^2. 
%     \]

Now we upperbound the second term in the RHS of equation \ref{mainN2}, 

\begin{align*}
&\norm{\frac{1}{S}\sum_{i=1}^S \Big ( f_{\w}(\x_i) - f_{\w_t}(\x_i) \Big)\M\x_i} = \frac{1}{wS}\norm{\sum_{i=1,j=1}^{w,S} \Big ( \sigma \Big (  \langle \A_i^\top \w , \x_j \rangle \Big ) - \sigma \Big (  \langle \A_i^\top \w_t, \x_j \rangle \Big )  \Big)\M \x_j}\\
&\leq \frac{L }{wS} \sum_{i=1,j=1}^{w,S} \vert \langle \A_i^\top( \w - \w_t) , \x_j \rangle \vert \norm{\M \x_j} \leq \frac{L }{wS} \sum_{i=1,j=1}^{w,S}  \norm{ \A_i^\top( \w - \w_t)}\times \norm{ \x_j} \times   \norm{\M \x_j}\\ 
&\leq {\rm B}^2 \sqrt{\lambda_{\max} \Big ( \M^\top \M \Big )} \times \frac{L}{w}  \times \norm{\w - \w_t} \sum_{i=1}^w \sqrt{\lambda_{\max} \Big ( \A_i \A_i^\top \Big )} 
\end{align*}

Thus combining the above two inequalities into the RHS of equation \ref{mainN2} we have, 

\begin{align*}
\text{Term 2 =} \norm{\frac{1}{S}\sum_{i=1}^S \Big (y_i - f_{\w_t}(\x_i) \Big ) \M \x_i}^2 \leq &\beta^2 + 2\beta \times \frac{{\rm B}^2 L}{w} \times \norm{\w - \w_t}  \sqrt{\lambda_{\max} \Big ( \M^\top \M \Big )} \Big ( \sum_{i=1}^w \sqrt{\lambda_{\max} \Big ( \A_i \A_i^\top \Big )} \Big )  \\
&+ {\rm B}^2 \lambda_{\max} \Big ( \M^\top \M \Big )  \times \tilde{L}_S(h_t) 
\end{align*}

Combining the above and equation \ref{term1} into the RHS of equation \ref{mainN} we get, 

\begin{align*}
    &\norm{\w_t - \w}^2 - \norm{\w_{t+1} - \w}^2\\
    &\geq -4\frac{\eta \beta \norm{\w-\w_t}}{w}  + 4\frac{ \eta (1+\alpha)}{2S}  \Big [ (\w - \w_t)^\top \Big ( \bar{\A} \tilde{\Sigma}  \M^\top \Big )  (\w - \w_t) \Big ] \\
    &-\Big ( \frac{2\eta}{w} \Big )^2 \Bigg ( \beta^2 + 2\beta \times \frac{{\rm B}^2 L}{w} \times \norm{\w - \w_t}  \sqrt{\lambda_{\max} \Big ( \M^\top \M \Big )} \Big ( \sum_{i=1}^w \sqrt{\lambda_{\max} \Big ( \A_i \A_i^\top \Big )} \Big )  + {\rm B}^2 \lambda_{\max} \Big ( \M^\top \M \Big )  \times \tilde{L}_S(h_t) \Bigg )
\end{align*}

which rearranges to the lemma we set out to prove. 

% \begin{align*}
%     \norm{\w_{t+1} - \w}^2 \leq &\norm{\w_t - \w}^2  - 4\frac{ \eta (1+\alpha)}{2S}  \Big [ (\w - \w_t)^\top \Big ( \bar{\A} \tilde{\Sigma}  \M^\top \Big )  (\w - \w_t) \Big ] \\
%     &+4\frac{\eta \beta \norm{\w-\w_t}}{w}\\
%     &+ \Big ( \frac{2\eta}{w} \Big )^2 \Bigg ( \beta^2 + 2\beta \times \frac{{\rm B}^2 L}{w} \times \norm{\w - \w_t}  \sqrt{\lambda_{\max} \Big ( \M^\top \M \Big )} \Big ( \sum_{i=1}^S \sqrt{\lambda_{\max} \Big ( \A_i \A_i^\top \Big )} \Big )  + {\rm B}^2 \lambda_{\max} \Big ( \M^\top \M \Big )  \times \tilde{L}_S(h_t) \Bigg )
% \end{align*}

%\qedsymbol
\end{proof}

%\newpage 
\begin{lemma}\label{discretesym}
Suppose $S := \{ (\x_i,y_i) \mid i=1,\ldots,S \}$ is a set if tuples  such that the set $S_\x := (\x_i)_{i=1,\ldots,S}$ is invariant under replacing each $\x_i$ with $-\x_i$. (Note that this does not enforce the label associated with $\x_i$ to have any relation to the label associated to $-\x_i$.). 
~\\ ~\\ 
Then for any $\A, \M \in \R^{r \times n}$ and $\z_1, \z_2 \in \R^{r}$ and $\forall i, \x_i \in \R^n$ and $\sigma : \R \rightarrow \R$ mapping, $x \mapsto x\mathbf{1}_{x\geq 0} + \alpha x\mathbf{1}_{x\leq 0}$ for some $\alpha >0$ we have, 

\[ \sum_{i=1}^S  \sigma \Big ( \langle \A^\top \z_1 , \x_i \rangle \Big )  \Big \langle M\x_i, \z_2 \Big \rangle = \frac{1+\alpha}{2} \z_1^\top \Big ( \A \tilde{\Sigma}  M^\top \Big ) \z_2  \] 

where we have defined, $\tilde{\Sigma} := \Big [ \sum_{i=1}^S  \x_i \x_i^\top \Big ]$
\end{lemma}

\begin{proof} 
By the assumed symmetry of the set $S_\x$ we have, 

\begin{align*}
&\sum_{i=1}^S  \sigma \Big ( \langle \A^\top \z_1 , \x_i \rangle \Big )  \Big \langle \M\x_i, \z_2 \Big \rangle = \sum_{i=1}^S  \sigma \Big ( - \langle \A^\top \z_1 , \x_i \rangle \Big )  \Big \langle - \M\x_i, \z_2 \Big \rangle \\
\implies &2\sum_{i=1}^S  \sigma \Big ( \langle \A^\top \z_1 , \x_i \rangle \Big )  \Big \langle \M\x_i, \z_2 \Big \rangle =  \sum_{i=1}^S  \Big [ \sigma \Big (  \langle \A^\top \z_1 , \x_i \rangle \Big )  \Big \langle  \M\x_i, \z_2 \Big \rangle  + \sigma \Big ( - \langle \A^\top \z_1 , \x_i \rangle \Big )  \Big \langle - \M\x_i, \z_2 \Big \rangle  \Big ]\\  
\implies &2\sum_{i=1}^S  \sigma \Big ( \langle \A^\top \z_1 , \x_i \rangle \Big )  \Big \langle \M\x_i, \z_2 \Big \rangle =  \sum_{i=1}^S  \Big [ \Big \{ \sigma \Big ( \langle \A^\top \z_1 , \x_i \rangle \Big )   - \sigma \Big ( - \langle \A^\top \z_1 , \x_i \rangle \Big )  \Big \} \Big \langle \M\x_i, \z_2 \Big \rangle  \Big ] 
\end{align*}

Note that  $\forall p \geq 0 \implies \sigma(p) = p$ and $\forall p <0 \implies \sigma(p) = \alpha p$. Thus it follows that $ \forall p \geq 0 \implies \sigma(p) - \sigma(-p) = p - \alpha(-p) = (1+\alpha)p$ and  $\forall p<0 \implies \sigma(p) - \sigma(-p) = \alpha p - (-p) = (1+\alpha)p$. Substituting this above we have,

\begin{align*}
2\sum_{i=1}^S  \sigma \Big ( \langle \A^\top \z_1 , \x_i \rangle \Big )  \Big \langle \M\x_i, \z_2 \Big \rangle &=  (1+\alpha) \sum_{i=1}^S  \Big [ \Big \{ \Big \langle \A^\top \z_1 , \x_i \Big \rangle  \Big \} \Big \langle \M\x_i, \z_2 \Big \rangle  \Big ] =  (1+\alpha) ( \A^\top \z_1)^\top \Big [ \sum_{i=1}^S  \x_i \x_i^\top \Big ]   \M^\top \z_2 \\
&= (1+\alpha)  \z_1^\top \Big ( \A \tilde{\Sigma}  M^\top \Big ) \z_2  
\end{align*}
\end{proof}
